# Supplementary material for: GenSQL: A Probabilistic Programming System for Querying Generative Models of Database Tables
Source: arXiv:2406.15652 source file (2024-06-21)
Supplement: Supplementary file 1 [file proofs.tex]

\section{Proofs}
\label{sec:proofs}

\printProofs
